# Supplementary material for: Determining damping terms in fractional wave equations
Source: arXiv:2112.00080 source file (2022-04-11)
Supplement: Supplementary file 1 [file appendix.tex]

\section*{Appendix}
\begin{lemma}\label{lem:nonzerocoeff}
For $c\in C^2(0,L)$ and any $s\in(\frac12+2(\mu+\nu),1)$, the function constructed as 
$f(x(\xi))=\sqrt{c(x(\xi))} \sum_{n=1}^\infty n^{-s} \phi_n^0(\xi)$ lies in $\dot{H}^{2(\mu+\nu)}$ and satisfies 
\[
\langle f,\varphi_k\rangle_{L^2_{1/c^2}}  \geq \underline{c}k^{-s} \mbox{ for all }k\in\mathbb{N}\,.
\]
\end{lemma}
\begin{proof}
Indeed, setting $C_s=\left(\sum_{n=1}^\infty n^{-2s}\right)^{1/2}$, by using the Cauchy-Schwarz inequality and the eigenfunction estimate %Lemma \ref{lem:slp_estimates} in fde-lect
$\|\phi_n^0 -\phi_n^q\|_{L^2}\leq\bar{C}n^{-1}\|q\|_{L^2}$ we have, for any $k$ 
\[
\begin{aligned}
|\langle f,\varphi_k\rangle_{L^2_{1/c^2}}| 
&= |\int_0^{\xi(L)} f(x(\xi)) c(x(\xi))^{-1/2} \phi_k^q(\xi)\, d\xi|\\
&=|\sum_{n=1}^\infty n^{-s} \langle \phi_k^q, \phi_n^0\rangle_{L^2}|
=|k^{-s}+\sum_{n=1}^\infty n^{-s}\langle \phi_k^q-\phi_k^0, \phi_n^0\rangle|\\
&\geq k^{-s}-C_s\, \|\phi_k^q-\phi_k^0\|_{L^2(\Omega)}
\geq k^{-s}-\bar{C}C_s\, k^{-1}\,.
\end{aligned}
\]
\end{proof}
Unfortunately this is only an existence result, since the reconstruction requires knowledge of $c$.

A simple substitute without any constraints on the level of smoothness (but again, just an existence result without practical computability) is
\begin{lemma}\label{lem:nonzerocoeff_simple}
For any $s>0$, $\epsilon>0$, the function 
$f(x)=c(x)^2\sum_{n=1}^\infty \lambda_n^{-s} n^{-(\frac12+\epsilon)} \varphi_n(x)$ lies in $\dot{H}^{s}$ and satisfies 
$\langle f,\varphi_k\rangle_{L^2_{1/c^2}}  \geq \lambda_n^{-s} n^{-(\frac12+\epsilon)} $ for all $k\in\mathbb{N}$.
\end{lemma}

\footnote{\textcolor{blue}{This seems a quite short appendix, can it be integrated into
the main body of the text?  It is not a major issue.}
\textcolor{cyan}{I put it into the appendix because I am not so sure whether it is really so useful for our purposes - maybe we can talk about completely removing this or just keep Lemma~\eqref{lem:nonzerocoeff_simple} in the main body of the text}}
